# Supplementary material for: CheXbert: Combining Automatic Labelers and Expert Annotations for Accurate Radiology Report Labeling Using BERT
Source: arXiv:2004.09167 source file (2020-10-18)
Supplement: Supplementary file 1 [file chexbert_vs_chexpert.tex]

\begin{table*}[h!]
\caption{\label{tab:chexbert_vs_chexpert} This table shows a side-by-side comparison of the weighted F1 scores for CheXpert and CheXbert as well as improvements in F1 score for CheXbert on the MIMIC-CXR test set. Confidence intervals for each of the columns were generated using the bootstrap method.}
\fontfamily{cmss}\selectfont
\begin{tabular}{l|ccc}
                  & \multicolumn{3}{c}{F1 (95\% CI)}                                     \\
Category          & CheXpert             & CheXbert             & Improvement            \\ \hline
Pleural Other     & 0.478 (0.321, 0.617) & 0.652 (0.477, 0.792) & 0.174 (0.084, 0.287)   \\
Pneumonia         & 0.684 (0.626, 0.742) & 0.797 (0.748, 0.845) & 0.113 (0.061, 0.162)   \\
Fracture          & 0.671 (0.509, 0.810) & 0.782 (0.645, 0.892) & 0.111 (0.017, 0.215)   \\
Consolidation     & 0.772 (0.679, 0.857) & 0.855 (0.782, 0.916) & 0.083 (0.000, 0.163)  \\
No Finding        & 0.543 (0.396, 0.659) & 0.608 (0.448, 0.721) & 0.065 (-0.026, 0.143)  \\ \hline
Pneumothorax      & 0.882 (0.841, 0.921) & 0.937 (0.903, 0.967) & 0.055 (0.020, 0.090)   \\
Enlarged Cardiom. & 0.613 (0.528, 0.691) & 0.666 (0.579, 0.739) & 0.053 (-0.016, 0.123)  \\
Cardiomegaly      & 0.764 (0.707, 0.815) & 0.810 (0.760, 0.856) & 0.046 (0.015, 0.082)   \\
Edema             & 0.864 (0.827, 0.901) & 0.887 (0.849, 0.920) & 0.023 (-0.002, 0.050)  \\
Lung Lesion       & 0.683 (0.570, 0.793) & 0.689 (0.573, 0.798) & 0.006 (-0.037, 0.044)  \\
Support Devices   & 0.867 (0.831, 0.903) & 0.873 (0.837, 0.907) & 0.006 (-0.011, 0.022)  \\
Atelectasis       & 0.917 (0.882, 0.951) & 0.919 (0.887, 0.949) & 0.002 (-0.031, 0.038)  \\
Pleural Effusion  & 0.905 (0.877, 0.932) & 0.904 (0.875, 0.931) & -0.001 (-0.019, 0.014) \\
Lung Opacity      & 0.762 (0.709, 0.809) & 0.751 (0.698, 0.800) & -0.011 (-0.048, 0.025) \\
Average           & 0.743 (0.719, 0.764) & 0.795 (0.772, 0.815) & 0.052 (0.037, 0.067)   \\ \hline
\end{tabular}
\end{table*}
